# Supplementary material for: LiDARTouch: Monocular metric depth estimation with a few-beam LiDAR
Source: arXiv:2109.03569 source file (2022-11-25)
Supplement: Supplementary file 1 [file acmnet.tex]

\begin{tikzpicture}[trim axis left, trim axis right]
% manual link https://ftp.cc.uoc.gr/mirrors/CTAN/graphics/pgf/contrib/pgfplots/doc/pgfplots.pdf
    \begin{axis}[
        % cycle list https://tex.stackexchange.com/questions/170221/pgfplots-line-colors
        % link to color palette: http://www.traag.net/wp/wp-content/uploads/2014/06/display_colors1.png
        % load a color `cycle list' from the `colorbrewer' library
        cycle list/Set1-3,
        % define fill color for the marker
        mark list fill={.!40!white},
        % create new `cycle list` from existing `cycle list`
        cycle multiindex* list={
            Set1-3
                \nextlist
            my marks
                \nextlist
            [3 of]linestyles
                \nextlist
            very thick
                \nextlist
        },
        legend cell align={left}, % align legend on the left
        xlabel=\textbf{Threshold $\tau$},
        ylabel=\textbf{CDR} (in \%),
        %ylabel near ticks,
        ylabel style={yshift=-10pt},
        ymode=log,
        log ticks with fixed point,
        ytick pos=left,
        xlabel style={yshift=3pt},
        xtick pos=bottom,
        xtick=data,
        x tick label style = {font = \small, align = center},%, rotate = 70},
        grid=major,
        xmajorgrids=false,
        grid style=dashed,
        legend style={
            at={(0.44,1.38)},
            draw=none, % removes legend border
            anchor=north,legend columns=2,
        },
	    scale only axis,height=3cm,width=0.85\columnwidth,
        ]
        
    \addplot plot coordinates {
        (0.1, 38.96)
        (0.2, 18.26)
        (0.3, 11.72)
        (0.4, 8.52)
        (0.5, 5.02)
        (0.6, 3.65)
        (0.7, 2.89)
        (0.8, 2.59)
        (0.9, 1.37)
        (1, 1.07)
    };
    \addlegendentry{Monodepth2 w/ IMU sup.}
    
    \addplot plot coordinates {
        (0.1, 33.18)
        (0.2, 15.82)
        (0.3, 7.00)
        (0.4, 2.13)
        (0.5, 0.6)
        (0.6, 0.15)
        (0.7, 0)
        (0.8, 0)
        (0.9, 0)
        (1, 0)
    };
    \addlegendentry{ACMNet$^{\textit{P}}\PnP$}
    
    \pgfplotsset{cycle list shift=+3} 
    \addplot+[solid] plot coordinates {
        (0.1, 13.09)
        (0.2, 1.67)
        (0.3, 0.15)
        (0.4, 0.15)
        (0.5, 0.00)
        (0.6, 0.00)
        (0.7, 0.00)
        (0.8, 0.00)
        (0.9, 0.00)
        (1, 0.00)
    };
    \addlegendentry{\ssACMNet}

    \end{axis}
\end{tikzpicture}
