# Supplementary material for: LiDARTouch: Monocular metric depth estimation with a few-beam LiDAR
Source: arXiv:2109.03569 source file (2022-11-25)
Supplement: Supplementary file 2 [file aggregate.tex]

\begin{figure*}[]
    \centering
    \begin{subfigure}[]{0.49\textwidth}
        \input{figures/inf_depth_study_appendix/acmnet}
    \end{subfigure}%
    \hfill
    \begin{subfigure}[]{0.49\textwidth}
        \input{figures/inf_depth_study_appendix/md2l}
    \end{subfigure}
    \\
    \begin{subfigure}[]{0.49\textwidth}
        \input{figures/inf_depth_study_appendix/nlspn}
    \end{subfigure}%
    \hfill
    \begin{subfigure}[]{0.49\textwidth}
        \input{figures/inf_depth_study_appendix/s2d}
    \end{subfigure}

\caption{\textbf{Plot of the CDR metric for various thresholds $\tau$.} $y$-axis is log-scaled.}
\label{fig:inf_depth_study_appendix}
\end{figure*}
